# Supplementary material for: A spectral element solution of the Poisson equation with shifted boundary polynomial corrections: influence of the surrogate to true boundary mapping and an asymptotically preserving Robin formulation
Source: arXiv:2310.17621 source file (2023-10-26)
Supplement: Supplementary file 1 [file Appendix.tex]

\appendix

\section{Weak formulation of Dirichlet boundary conditions - symmetric}\label{sec:appendix_symmetric}

\subsection{On a conformal boundary}\label{sec:appendix_symmetric_cbm}

In the body-fitting conformal boundary case, we have the symmetric version of the non-symmetrical weak formulation for Dirichlet boundary conditions in \eqref{eq:weak_cbm_bilinear_dbc} and \eqref{eq:weak_cbm_linear_dbc} as
\begin{align}
    a\langle u,v \rangle_{\Gamma_D} &= \tau (u,v)_{\Gamma_D} -  (\nabla u \cdot \boldsymbol{n},v)_{\Gamma_D} - (\nabla v \cdot \boldsymbol{n},u)_{\Gamma_D}, 
\end{align}
and
\begin{align}
    b\langle v \rangle_{\Gamma_D} &= \tau (u_D,v)_{\Gamma_D} - (\nabla v \cdot \boldsymbol{n},u_D)_{\Gamma_D}. 
\end{align}




\subsection{On a shifted boundary - with a polynomial correction}\label{sec:appendix_symmetric_sbm}

In the unfitted case for the SBM with a polynomial correction, we have the symmetrical form of \eqref{eq:weak_sbm_bilinear_dbc_final} and \eqref{eq:weak_sbm_linear_dbc_final} as
\begin{align}
    a\langle u,v \rangle_{\overline{\Gamma}_D} &= \tau (u(\boldsymbol{x}),v)_{\overline{\Gamma}_D} - (\nabla u \cdot \overline{\boldsymbol{n}},v)_{\overline{\Gamma}_D} - (\nabla v \cdot \overline{\boldsymbol{n}},u(\boldsymbol{x}))_{\overline{\Gamma}_D}, \label{eq:weak_sbm_bilinear_dbc_final_sym}
\end{align}
and
\begin{align}
    b\langle v \rangle_{\overline{\Gamma}_D} &= \tau ({u}_D,v)_{\overline{\Gamma}_D} - (\nabla v \cdot \overline{\boldsymbol{n}},u_D)_{\overline{\Gamma}_D}. \label{eq:weak_sbm_linear_dbc_final_sym}
\end{align}











\section{Polynomial correction on the Robin boundary}\label{sec:appendix_robin}

From the weak formulation in \eqref{eq:weak_sbm_1} and the Robin-associated non-symmetrical contributions to the bi-linear and linear forms in \eqref{eq:weak_sbm_bilinear_rbc_1} and \eqref{eq:weak_sbm_linear_rbc_1}, we have that
\begin{align}
    a \langle u,v \rangle_{\overline{\Gamma}_R} &= \frac{1}{\varepsilon + \gamma} (u,v)_{\overline{\Gamma}_R} - \frac{\gamma}{\varepsilon + \gamma} (\nabla u \cdot \overline{\boldsymbol{n}},v)_{\overline{\Gamma}_R}, \\
    b\langle v \rangle_{\overline{\Gamma}_R} &= \frac{1}{\varepsilon + \gamma} (\overline{u}_{RD},v)_{\overline{\Gamma}_R} + \frac{\varepsilon}{\varepsilon + \gamma} (\overline{u}_{RN},v)_{\overline{\Gamma}_R}.
\end{align}

Applying the same decomposition of the surrogate normal, as for the Neumann boundary: $\overline{\boldsymbol{n}} = \boldsymbol{n}(\overline{\boldsymbol{n}} \cdot \boldsymbol{n}) + \boldsymbol{t}(\overline{\boldsymbol{n}} \cdot \boldsymbol{t})$. From this
\begin{equation}\label{eq:app_5}
    (\overline{u}_{RN},v)_{\overline{\Gamma}_R} = (\nabla u(\overline{\boldsymbol{x}}) \cdot \overline{\boldsymbol{n}},v)_{\overline{\Gamma}_R} = (\overline{\boldsymbol{n}} \cdot \boldsymbol{n}) (\nabla u(\overline{\boldsymbol{x}}) \cdot \boldsymbol{n},v)_{\overline{\Gamma}_R}  + (\overline{\boldsymbol{n}} \cdot \boldsymbol{t}) (\nabla u(\overline{\boldsymbol{x}}) \cdot \boldsymbol{t},v)_{\overline{\Gamma}_R}.
\end{equation}

Then applying a $k$'th order truncated multivariant Taylor series expansion of $u_{RD}(\boldsymbol{x})$ and $u_{RN}(\boldsymbol{x})$ on $\Gamma$ around the point $\overline{\boldsymbol{x}} \in \overline{\Gamma}$
\begin{align}
    u_{RD}(\boldsymbol{x}) &= u(\boldsymbol{\overline{x}}) + \mathcal{D}^k_{RD} , \quad \text{where} \quad \mathcal{D}^k_{RD} = \sum_{\alpha = 1}^k \frac{1}{\alpha !}   \left ( \nabla^{\alpha}  \right) \left ( u \right )(\boldsymbol{\overline{x}}) \boldsymbol{d}(\boldsymbol{\overline{x}})^{\alpha}, \\
    u_{RN}(\boldsymbol{x}) &= \nabla u(\boldsymbol{\overline{x}}) \cdot \boldsymbol{n} + \mathcal{D}^k_{RN}, \quad \text{where} \quad \mathcal{D}^k_{RN} = \sum_{\alpha = 1}^k \frac{1}{\alpha !}   \left ( \nabla^{\alpha}  \right) \left (\nabla u \cdot \boldsymbol{n} \right )(\boldsymbol{\overline{x}}) \boldsymbol{d}(\boldsymbol{\overline{x}})^{\alpha}, 
\end{align}
which gives expressions for $u(\boldsymbol{\overline{x}})$ and $\nabla u(\boldsymbol{\overline{x}}) \cdot \boldsymbol{n}$ as
\begin{align}
   u(\boldsymbol{\overline{x}})  &=   u_{RD}(\boldsymbol{x})  - \mathcal{D}^k_{RD}, \label{eq:app_2}\\
   \nabla u(\boldsymbol{\overline{x}}) \cdot \boldsymbol{n}  &=  u_{RN}(\boldsymbol{x}) - \mathcal{D}^k_{RN}. \label{eq:app_4}
\end{align}

Now, as for the Dirichlet and Neumann cases, we will again consider an exact $k$'th order Taylor polynomial expansion series of $u (\boldsymbol{x})$ and $\nabla u (\boldsymbol{x}) \cdot \boldsymbol{n}$ on $\Gamma$ around the point $\overline{\boldsymbol{x}} \in \overline{\Gamma}$
\begin{align}
     u(\boldsymbol{x}) =  u(\overline{\boldsymbol{x}}) + \mathcal{D}^k_{RD} \quad &\Longleftrightarrow \quad \mathcal{D}^k_{RD} =  u(\boldsymbol{x}) -  u(\overline{\boldsymbol{x}}),\label{eq:app_1} \\
    \nabla u(\boldsymbol{x}) \cdot \boldsymbol{n} = \nabla u(\overline{\boldsymbol{x}}) \cdot \boldsymbol{n} + \mathcal{D}^k_{RN} \quad &\Longleftrightarrow \quad \mathcal{D}^k_{RN} = \nabla u(\boldsymbol{x}) \cdot \boldsymbol{n} - \nabla u(\overline{\boldsymbol{x}}) \cdot \boldsymbol{n}. \label{eq:app_3}
\end{align}

Finally, combining \eqref{eq:app_1} with \eqref{eq:app_2} and \eqref{eq:app_3} with \eqref{eq:app_4} gives expressions for the surrogate boundary conditions as
\begin{align}
    u(\boldsymbol{\overline{x}}) &= u_{RD}(\boldsymbol{x}) - u(\boldsymbol{x}) + u(\boldsymbol{\overline{x}}), \\
       \nabla u(\boldsymbol{\overline{x}}) \cdot \boldsymbol{n} &= u_{RN}(\boldsymbol{x}) - \nabla u(\boldsymbol{x}) \cdot \boldsymbol{n} + \nabla u(\overline{\boldsymbol{x}}) \cdot \boldsymbol{n}.
\end{align}

And putting this together with the decomposition in \eqref{eq:app_5}, we arrive at the following expressions for the bi-linear and linear forms originally given in \eqref{eq:weak_sbm_bilinear_rbc_1} and \eqref{eq:weak_sbm_linear_rbc_1}
\begin{align}
a \langle u,v \rangle_{\overline{\Gamma}_R} &= \frac{1}{\varepsilon + \gamma} (u(\boldsymbol{x}),v)_{\overline{\Gamma}_R} - \frac{\gamma}{\varepsilon + \gamma} (\nabla u \cdot \overline{\boldsymbol{n}},v)_{\overline{\Gamma}_R} + \frac{(\overline{\boldsymbol{n}} \cdot \boldsymbol{n})\varepsilon}{\varepsilon + \gamma} (\nabla u({\boldsymbol{x}}) \cdot \boldsymbol{n} - \nabla u \cdot \boldsymbol{n},v)_{\overline{\Gamma}_R}  -\frac{(\overline{\boldsymbol{n}} \cdot \boldsymbol{t})\varepsilon}{\varepsilon + \gamma} (\nabla u \cdot \boldsymbol{t},v)_{\overline{\Gamma}_R} \\
b \langle v \rangle_{\overline{\Gamma}_R} &= \frac{1}{\varepsilon + \gamma} (u_{RD},v)_{\overline{\Gamma}_R} + \frac{(\overline{\boldsymbol{n}} \cdot \boldsymbol{n})\varepsilon}{\varepsilon + \gamma} (u_{RN},v)_{\overline{\Gamma}_R}.
\end{align}

%% OLD:

% In the body-fitting conformal boundary case, we have the symmetric version of the non-symmetrical weak formulation outlined in \eqref{eq:weak_cbm} though \eqref{eq:weak_cbm_linear_rbc}. As always, the task is then to find $u \in C^1(\Omega)$ such that
% \begin{equation}
%     a \langle u,v \rangle = b\langle v \rangle, \label{eq:weak_cbm_sym}
% \end{equation}
% where the bi-linear and linear forms can be expanded, respectively, as
% \begin{align}
%     a\langle u,v \rangle &= a\langle u,v \rangle_{\Omega} + a\langle u,v \rangle_{\Gamma_D}+ a \langle u,v \rangle_{\Gamma_N} + a \langle u,v \rangle_{\Gamma_R}, \label{eq:weak_cbm_bilinear_sym} \\
%     a\langle u,v \rangle_{\Omega} &= (\nabla u, \nabla v)_{\Omega}, \label{eq:weak_cbm_bilinear_2d_sym}\\ 
%     a\langle u,v \rangle_{\Gamma_D} &= \tau (u,v)_{\Gamma_D} -  (\nabla u \cdot \boldsymbol{n},v)_{\Gamma_D} - (\nabla v \cdot \boldsymbol{n},u)_{\Gamma_D}, \label{eq:weak_cbm_bilinear_dbc_sym}\\
%     a \langle u,v \rangle_{\Gamma_N} &= 0, \label{eq:weak_cbm_bilinear_nbc_sym}\\
%     a \langle u,v \rangle_{\Gamma_R} &= \frac{1}{\varepsilon + \gamma} (u,v)_{\Gamma_R} - \frac{\gamma}{\varepsilon + \gamma} (\nabla u \cdot \boldsymbol{n},v)_{\Gamma_R} - \frac{\gamma}{\varepsilon + \gamma} (\nabla v \cdot \boldsymbol{n},u)_{\Gamma_R} - \frac{\varepsilon \gamma}{\varepsilon + \gamma} (\nabla v \cdot \boldsymbol{n},\nabla u \cdot \boldsymbol{n})_{\Gamma_R}, \label{eq:weak_cbm_bilinear_rbc_sym}
% \end{align}
% and
% \begin{align}
%     b\langle v \rangle &= b\langle v \rangle_{\Omega} + b\langle v \rangle_{\Gamma_D} + b \langle v \rangle_{\Gamma_N} + b\langle v \rangle_{\Gamma_R}, \label{eq:weak_cbm_linear_sym} \\
%     b\langle v \rangle_{\Omega} &= (f, v)_{\Omega}, \label{eq:weak_cbm_linear_2d_sym}\\
%     b\langle v \rangle_{\Gamma_D} &= \tau (u_D,v)_{\Gamma_D} - (\nabla v \cdot \boldsymbol{n},u_D)_{\Gamma_D}, \label{eq:weak_cbm_linear_dbc_sym}\\
%     b \langle v \rangle_{\Gamma_N} &= (u_N,v)_{\Gamma_N}, \label{eq:weak_cbm_linear_nbc_sym}\\
%     b\langle v \rangle_{\Gamma_R} &= \frac{1}{\varepsilon + \gamma} (u_{RD},v)_{\Gamma_R} + \frac{\varepsilon}{\varepsilon + \gamma} (u_{RN},v)_{\Gamma_R} - \frac{\gamma}{\varepsilon + \gamma} (\nabla v \cdot \boldsymbol{n},u_{RD})_{\Gamma_R} - \frac{\varepsilon \gamma}{\varepsilon + \gamma} (\nabla v \cdot \boldsymbol{n},u_{RN})_{\Gamma_R}. \label{eq:weak_cbm_linear_rbc_sym}
% \end{align}
