# Supplementary material for: A spectral element solution of the Poisson equation with shifted boundary polynomial corrections: influence of the surrogate to true boundary mapping and an asymptotically preserving Robin formulation
Source: arXiv:2310.17621 source file (2023-10-26)
Supplement: Supplementary file 2 [file Appendix_v2.tex]

\appendix

\newpage

\section{Figures for Dirichlet boundary conditions}\label{sec:appendix_neumann}

\subsection{\emph{p}-convergence and conditioning}

\begin{figure}[h]
    \centering \includegraphics{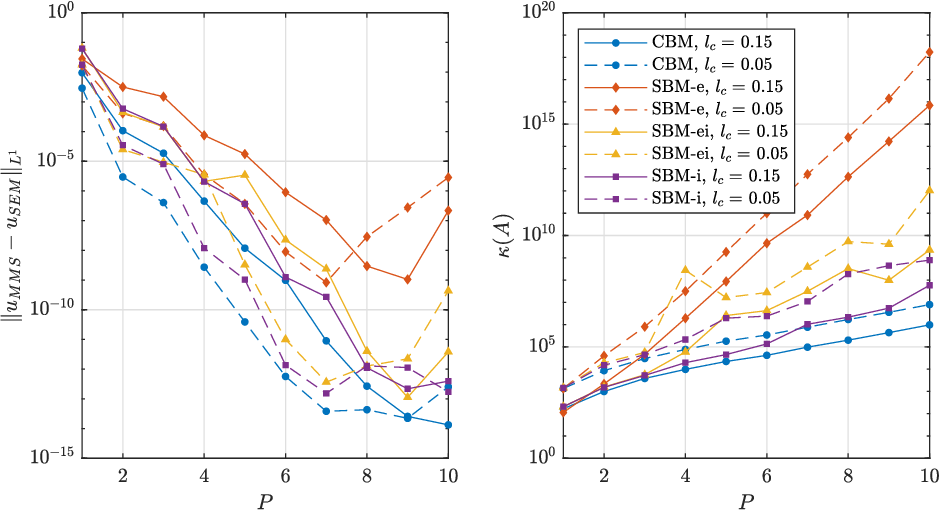}
    \caption{Left: $p$-convergence study with Neumann boundary conditions for CBM, SBM-e, SBM-ei, and SBM-i for two different meshes: $l_c = 0.15$ (full lines) and $l_c = 0.05$ (dashed lines). Right: Associated study of the matrix conditioning, $\kappa(\mathcal{A})$, for the same numerical setup.}
    \label{fig:P_convergence_non_sym_NBC}
\end{figure}

\newpage

\subsection{\emph{h}-convergence}

\begin{figure}[h]
    \centering
    \vspace{10mm}
    \includegraphics[scale = 0.9]{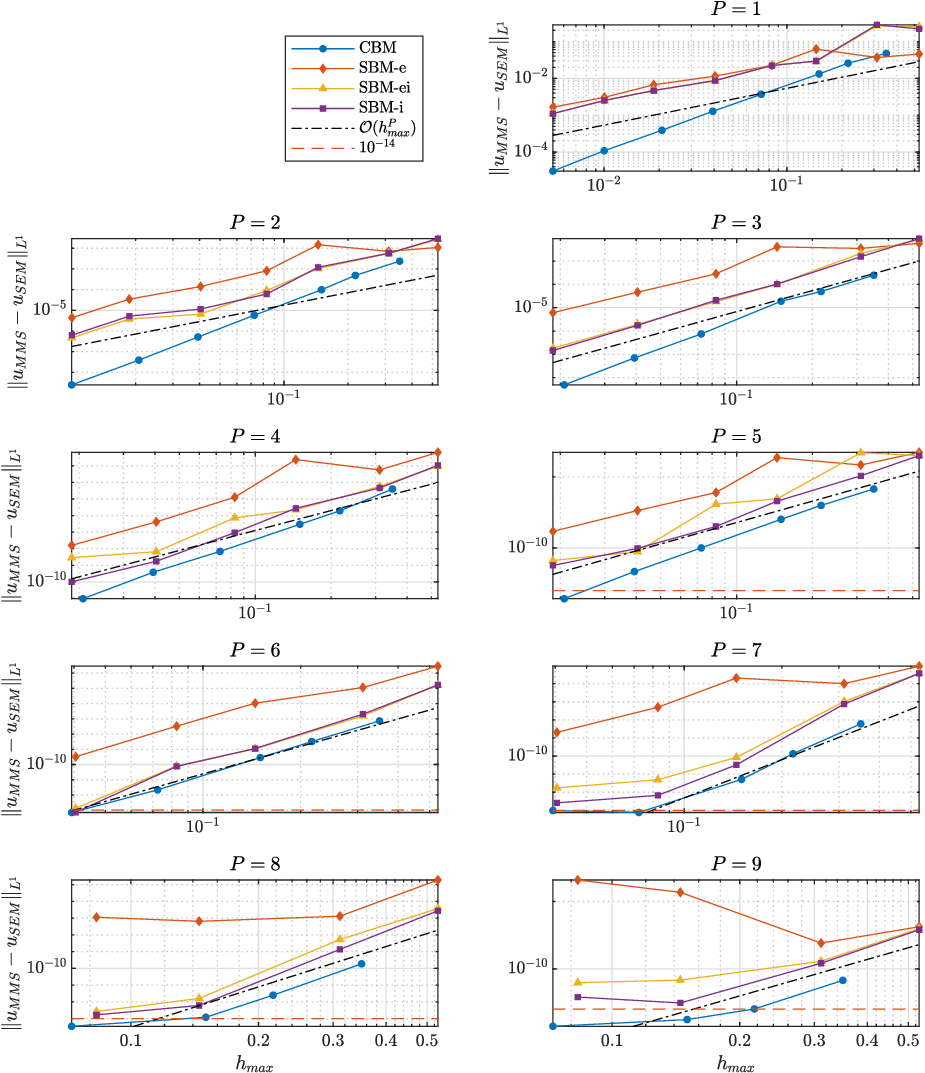}
    \caption{$h$-convergence study for $P \leq 9$ for Neumann boundary conditions for CBM, SBM-e, SBM-ei, and SBM-i.}
    \label{fig:h_convergence_non_sym_NBC}
\end{figure}

\newpage

\subsection{Conditioning under \emph{h}-convergence}

\begin{figure}[h]
    \centering
    \vspace{10mm}
    \includegraphics[scale = 0.9]{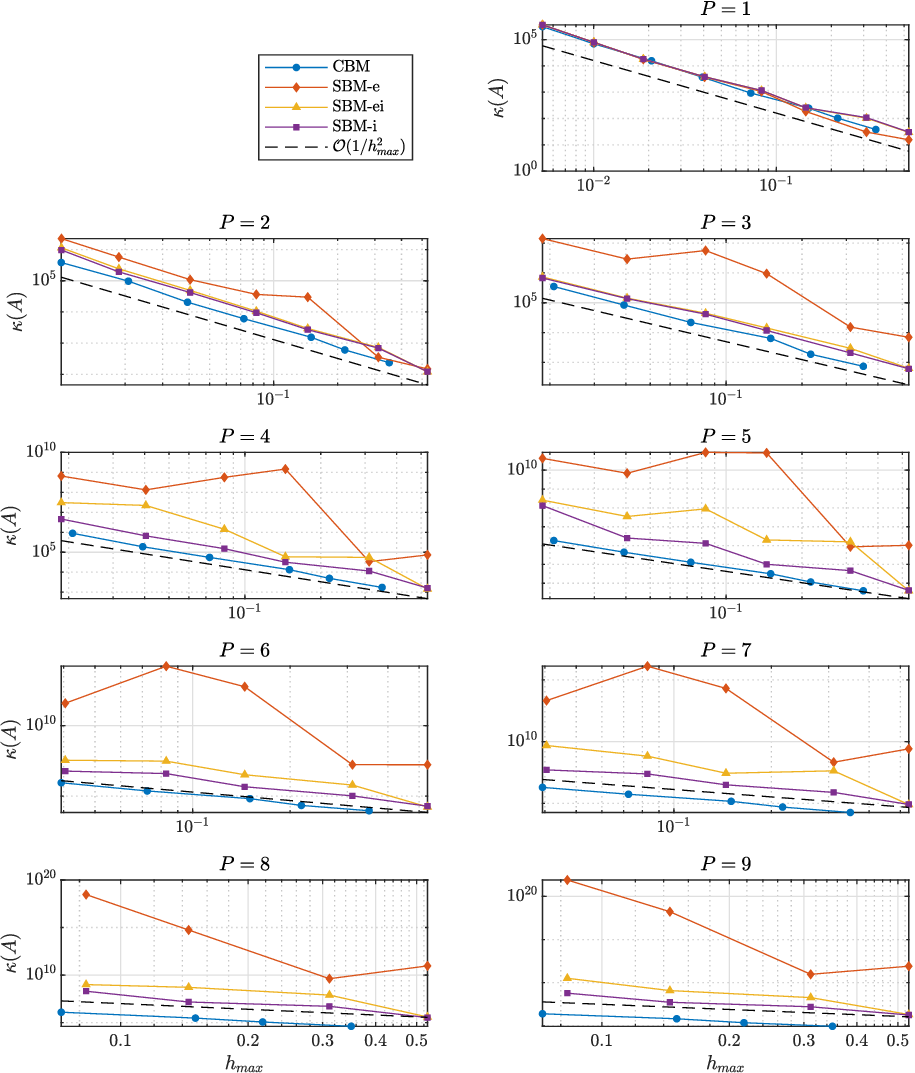}
    \caption{Study of matrix conditioning under $h$-refinement for $P \leq 9$ for Neumann boundary conditions for CBM, SBM-e, SBM-ei, and SBM-i. System matrices are from the study in Figure \ref{fig:h_convergence_non_sym_NBC}.}
    \label{fig:h_convergence_non_sym_NBC_cond_A}
\end{figure}

\newpage
